# Supplementary material for: Universal Critical Exponents of the Magnetic Domain Wall Depinning Transition
Source: arXiv:2101.06555 ancillary file (2021-07-15)
Supplement: Supplementary file 1 [file DepinningGdFeCo_SuppMaterial.pdf]

# Supplemental material of *Universal Critical Exponents of the Magnetic Domain Wall Depinning Transition*

L. J. Albornoz,<sup>1,2,3</sup> E. E. Ferrero,<sup>1</sup> A. B. Kolton,<sup>3,4</sup>

V. Jeudy,<sup>2</sup> S. Bustingorry,<sup>1</sup> and J. Curiale<sup>1,3</sup>

<sup>1</sup>*Instituto de Nanociencia y Nanotecnología,  
CNEA–CONICET, Centro Atómico Bariloche,*

*Av. E. Bustillo 9500 (R8402AGP),*

*San Carlos de Bariloche, Río Negro, Argentina.*

<sup>2</sup>*Université Paris-Saclay, CNRS, Laboratoire de Physique des Solides, 91405, Orsay, France.*

<sup>3</sup>*Instituto Balseiro, Universidad Nacional de Cuyo–CNEA, Centro Atómico Bariloche,  
Av. E. Bustillo 9500 (R8402AGP) San Carlos de Bariloche, Río Negro, Argentina.*

<sup>4</sup>*Centro Atómico Bariloche, Comisión Nacional de Energía Atómica (CNEA),  
Consejo Nacional de Investigaciones Científicas y Técnicas (CONICET),  
Av. E. Bustillo 9500 (R8402AGP) San Carlos de Bariloche, Río Negro, Argentina.*

(Dated: June 18, 2021)

## THERMAL ROUNDING OF THE DEPINNING TRANSITION

The conditions  $0 < H/H_d - 1 \ll 1$  and  $T/T_d \ll 1$  must be fulfilled in order to access the critical region at depinning. In this region the phenomenological formula for the thermal rounding of the depinning transition  $v(H, T) \approx (H/H_d - 1)^\beta G[(H/H_d - 1)^\beta / (T/T_d)^\psi]$ , with  $\psi \approx 0.15$  the thermal rounding exponent [1–3] holds. The expected asymptotic for  $G(x)$  in the critical regime  $T/T_d \ll 1$  and  $(H/H_d - 1) \ll 1$  is  $G(x) = \text{cst}$  for  $x \gtrsim 1$  and  $G(x) \sim x$  for  $x \ll 1$ . Therefore, in order to cleanly extract  $\beta$  from the zero-temperature depinning law  $v(H, T) \sim (H/H_d - 1)^\beta$  we need to assure  $x \equiv (H/H_d - 1)^\beta / (T/T_d)^\psi \gtrsim 1$ . This condition is fairly fulfilled by our temperatures ( $T/T_d \lesssim 0.002$ ) and fields ( $0.03 < H/H_d - 1 < 0.22$ ) fitting ranges.

## PROTOCOL USED FOR THE ANALYSIS OF THE DEPINNING TRANSITION

The depinning transition, formally defined at zero temperature, is described by the power-law vanishing of the moving interface velocity when the driving external field  $H$  approaches the depinning field  $H_d$  from above [1, 3–7]:

$$v(H, T \ll T_d) = v_0 \left( \frac{H - H_d}{H_d} \right)^\beta. \quad (1)$$

The velocity depinning exponent  $\beta$  gives the power-law growth of the domain wall velocity as a function of the external magnetic field  $H$  and  $v_0$  is a depinning velocity. Given this equation, we can fit  $\ln(v)$  as a function of  $\ln[(H - H_d)/H_d]$  to obtain  $\beta$  as the slope of the linear fit and  $\ln(v_0)$  as the intercept.

### Depinning transition with an independent $\beta$ for each temperature

To obtain the best set of values for each temperature, while fixing the  $H_d$  value, we fit the experimental results with only two free parameters. To find the most appropriate value of  $H_d$  and therefore that of  $\beta$  and  $v_0$  the following protocol was applied.

We first define a range of possible values of  $H_d$  for each considered temperature (10, 15, 20, 30, 40, 56 and 71 K). For each temperature, a field value  $H_{\min}$  exists below which we cannot define a mean DW velocity. Even if there is a range  $H < H_{\min}$  in which we can measure velocities, the DW displacement is not that smooth: Kerr images evidence tortuous

dynamics and eventually plastic events where DWs seem to break and small “islands” of opposite magnetization remain after the DW passage. We assume that  $H_d$  must be above  $H_{\min}$ . The other limit is given by  $H_{\max}$ , above that field the DW displacement is rather uniform; DW velocities are well defined and also relatively high:  $v \gtrsim 100$  m/s. In order to assure that all these fits will be performed considering the same number of data points, we only consider measured points with  $H > H_{\max}$  (full symbols on the right part of Fig. 1). Then, for each temperature we perform fits of  $\ln(v)$  vs.  $\ln[(H - H_d)/H_d]$  for different values of  $H_d$  in the range  $[H_{\min}, H_{\max}]$ . We seek for the  $H_d$  value in this range that maximizes the goodness of the fit, i.e., minimizes  $\chi^2 = \frac{1}{N} \sum \sigma_i^2 = \frac{1}{N} \sum \left( \frac{y_i - (a + bx_i)}{\delta y_i} \right)^2$ . Where  $x_i$ ,  $y_i$  and  $\delta y_i$  are the values of  $\ln[(H - H_d)/H_d]$ ,  $\ln(v)$  and the uncertainty in  $\ln(v)$ , respectively;  $a$  and  $b$  are the intercept and slope of the fit, and  $N$  is the number of data points for a given temperature. We finally calculate the estimated  $H_d(T)$  and its uncertainty by considering all the proposed  $H_d$  that verify  $\chi^2 < 1.1\chi_{\min}^2$  for the fit, with  $\chi_{\min}^2$  the minimum  $\chi^2$  value obtained in the range tested. In Fig. 1, left column, we show in combined plots  $\chi^2$  vs.  $H_d$  and  $\beta$  vs.  $H_d$ , in the ranges  $H_{\min} < H_d < H_{\max}$ , for each temperature analyzed. Limiting values  $1.1\chi_{\min}^2$  are shown as horizontal dotted lines, and the resulting  $H_d$  determinations are evidenced as a vertical red dashed line in each case, with its uncertainty indicated by a surrounding red-shaded region. In particular, the  $H_d$  value chosen for each  $T$  is the central value of the range in which  $\chi^2 < 1.1\chi_{\min}^2$ , and the uncertainty is half of its width. Once determined the  $H_d$  for each temperature, we calculate  $\beta$  and  $v_0$  by fitting Eq.1 with that particular  $H_d$ ; and their uncertainties are computed by considering their resulting values if we vary  $H_d$  in its own uncertainty range. Individual fits uncertainties were also taken into account. The left column of Fig. 1 also shows, the resulting value of  $\beta$  (blue dashed line), and its uncertainty (blue-shaded region). In the central column of Fig. 1 we plot  $\ln(v)$  vs.  $\ln[(H - H_d)/H_d]$  for different temperatures. In each plot, the dashed straight line correspond to Eq.1 with the  $\ln(v_0)$  and  $\beta$  values determined from the previous protocol. Finally, in the right column of Fig. 1 we show the same data as in the central column, but in a linear scale,  $v$  vs.  $\mu_0 H$ . For each temperature, the gray-shaded area is the range  $[H_{\min}, H_{\max}]$ , the red-dashed line is  $H_d$ , and the red-shaded area, its uncertainty.

The obtained values for  $\mu_0 H_d$ ,  $v_0$  and  $\beta$  are reported as a function of the temperature in Figure 2.  $H_d$  shows a non-monotonous behavior with  $T$ , with a minimum value for  $T = 30$  K. The velocity  $v_0$  increases a bit with increasing temperature. For  $\beta$ , the obtained

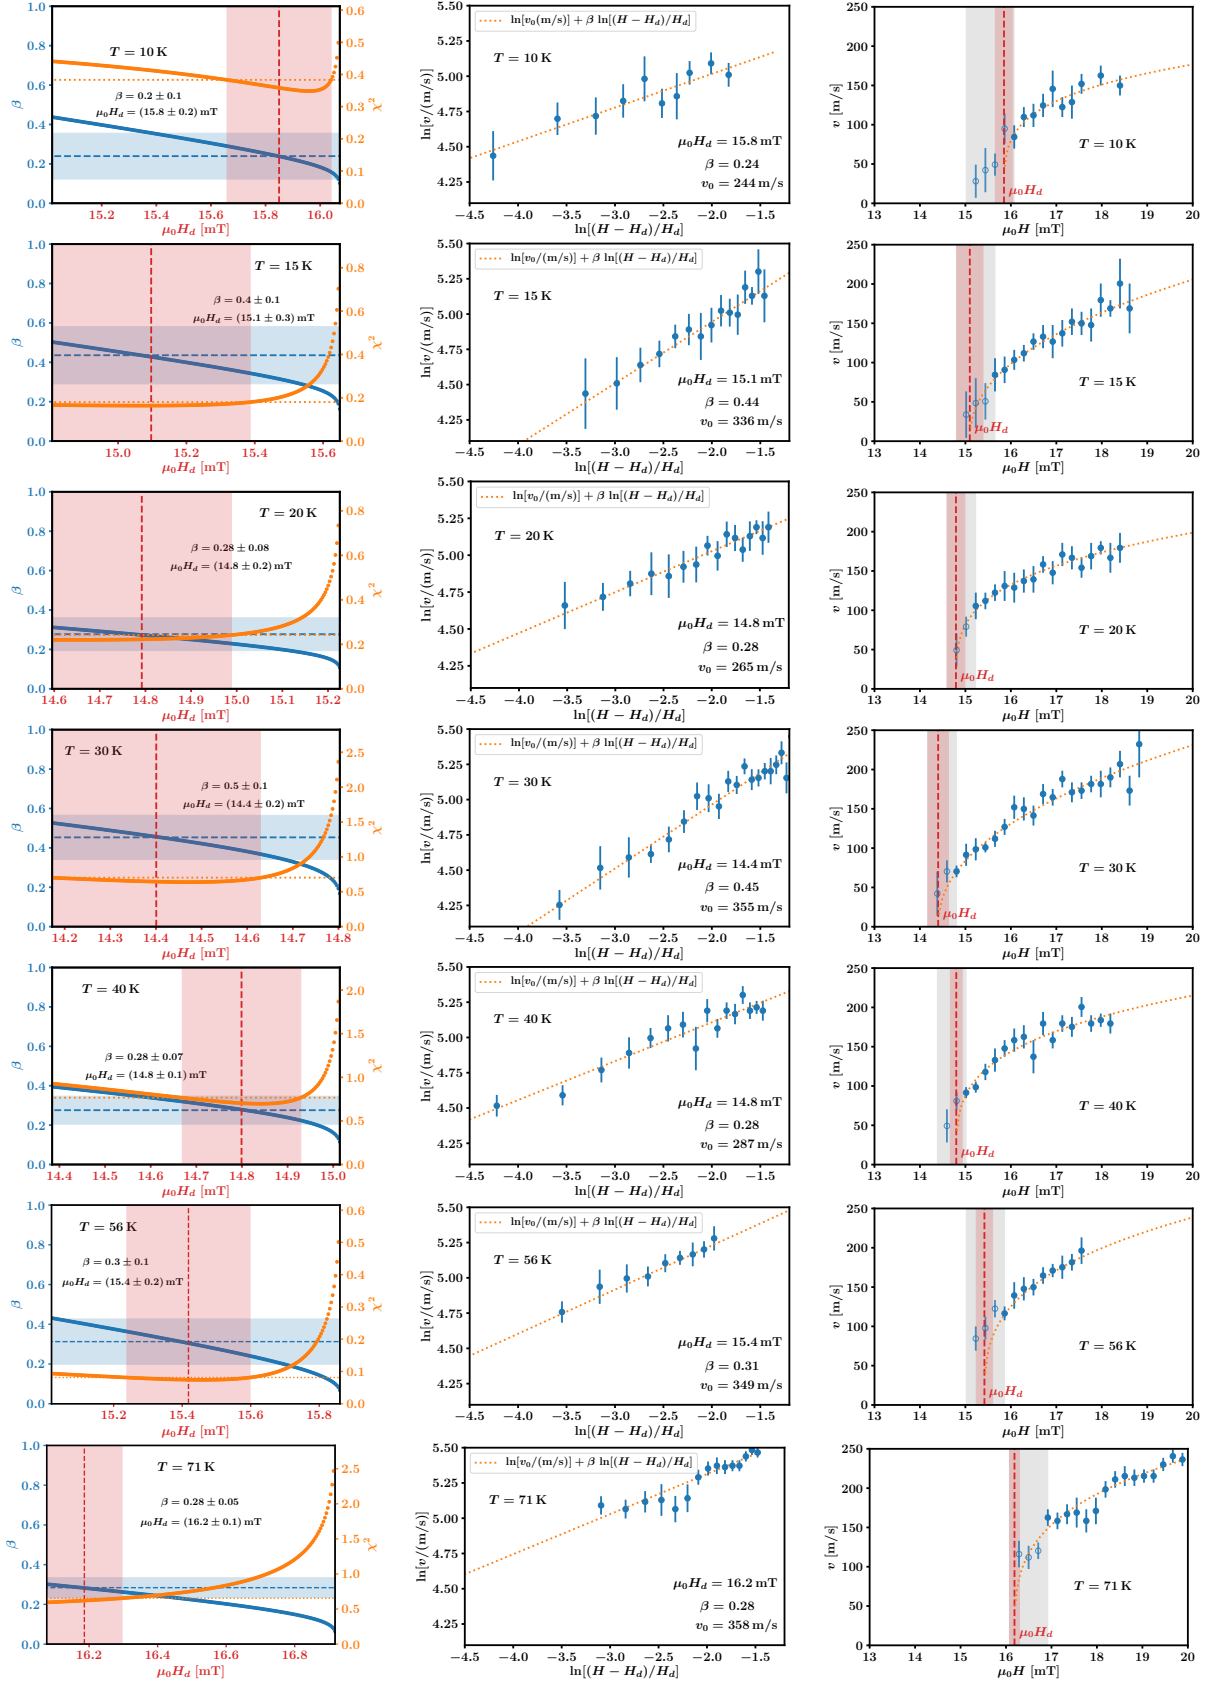

Figure 1. Analysis of the experimental results obtained in the temperature range  $10 \text{ K} \leq T \leq 71 \text{ K}$ . Left:  $\beta$  and  $\chi^2$  values as a function of the depinning field  $\mu_0 H_d$ .  $\mu_0 H_d$ ,  $\beta$  and its uncertainties are highlighted as dashed lines and shaded areas, respectively. Center and Right: Experimental results (blue dots) and resulting fit (orange dotted line) in a logarithmic and linear scale respectively.

values essentially present fluctuations around a mean value, indicated by a dotted line in Fig. 2. This strongly suggests that the obtained value of  $\beta$  can be described by a mean value ( $= 0.33 \pm 0.04$ ) over the explored temperature range  $10 \text{ K} \leq T \leq 71 \text{ K}$ .

### Depinning transition with $\beta$ as a global parameter

The same data were analysed with an alternative fitting method using the global fit tool of OriginLab. The procedure consists in a simultaneous fit of the whole set of curves obtained at different temperature, with  $\beta$  as a shared free (i.e., T-independent) parameter, and  $H_d$ , and  $v_0$  as free temperature dependent parameters. The obtained results for  $H_d$ , and  $v_0$  are reported in Figure 2 and are in good agreement with those deduced from the previous fitting method. The obtained value of  $\beta$  ( $= 0.33 \pm 0.04$ ) is also in good agreement with the mean value  $\beta$  ( $= 0.33 \pm 0.04$ ) deduced from the previous fitting method, which is a further evidence that the exponent  $\beta$  can be considered as temperature independent.

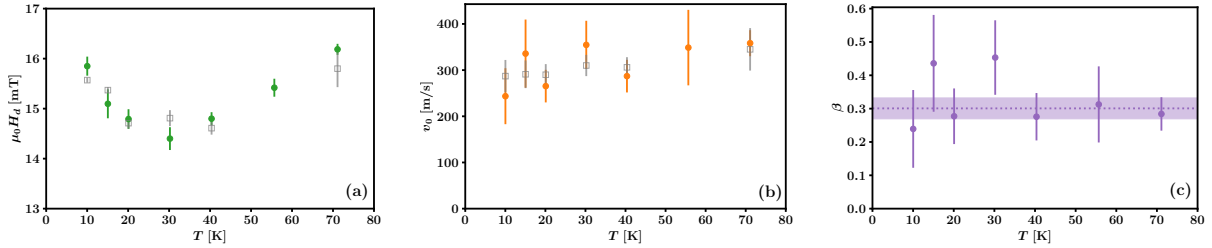

Figure 2.  $\mu_0 H_d$ ,  $v_0$  and  $\beta$  obtained values as a function of the temperature. Left:  $\mu_0 H_d$  values as determined by both protocol. Center:  $v_0$  values as determined by both protocol. Right: Velocity depinning exponent  $\beta$  as a function of temperature. Mean value is shown by the dotted line and their uncertainty as a shaded area.

### Depinning transition in other materials

Let us now discuss the compatibility of the obtained value of  $\beta$  with velocity curves obtained for other material. DWs systematically present an a-thermal depinning behavior as reflected by the universal function reported in Ref. [3]. However, due to thermal activation, the identification of the a-thermal depinning behaviour in a velocity-field characteristics is not direct. Indeed, upon increasing an applied magnetic field, the DW follows different

dynamical regimes, which are not straightforward to separate: thermally activated creep, depinning transition (which starts with a temperature dependent behavior and ends with an a-thermal behavior), crossover to the flow regimes, and flow regimes. Therefore, in order to perform an accurate global fit of Eq. 1 of the letter, some (reasonable) criteria have to be defined for the boundaries ( $H_{low}$ , and  $H_{high}$ ) the a-thermal depinning behaviour. As discussed in Ref. [3], ( $H_{low}$ ) is reached for  $x \gtrsim 0.8$ , with the lower boundary of the temperature dependent depinning transition coinciding with the upper boundary of the creep regime. For the values of  $H_{low}$ , we have simply used the values of  $H_d$  and  $T_d$ , reported in Ref. [8].

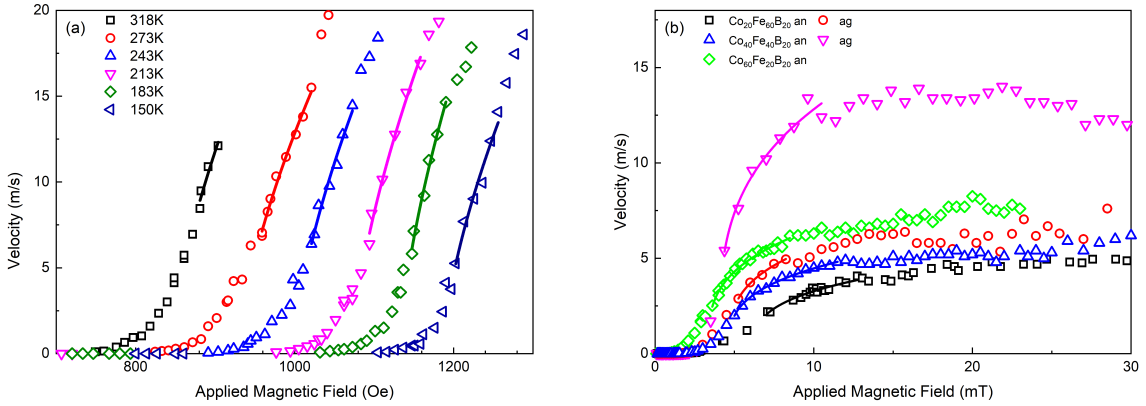

Figure 3. Domain-wall dynamics observed (a) in Au/Co/Au for different temperatures and (b) in Ta/CoFeB/MgO for different cobalt and iron concentrations and for as-grown (ag) and annealed (an) films. The data are taken from Ref. [3].

The upper boundary  $H_{high}$  is more difficult to determine since there exists no model to describe the shape of the crossover to the flow regimes. For Au/Co/Au, fitting all the data above  $H_{low}$  leads to a too large value of  $\beta$  ( $= 0.65 \pm 0.10$ ), which suggests that the crossover to the flow regimes is reached (see also the discussion in Ref. [3]). Eliminating the 2-3 points corresponding to the highest velocities (see Fig. 3(a)) leads to  $\beta = 0.31 \pm 0.04$  in agreement with the results obtained for GdFeCo. (Eliminating more points leads to an over parametrization of the fit.) For CoFeB (see Fig. 3(b)), the velocity-field characteristics present a long tail above the depinning transition and even a negative slope in the case of Co<sub>20</sub>Fe<sub>60</sub>B<sub>20</sub> (as grown) suggesting that the well-known plateau of the flow regime is reached. Fitting all the data above  $H_{low}$  leads (except for Co<sub>20</sub>Fe<sub>60</sub>B<sub>20</sub> (as grown)) to  $\beta = 0.17 \pm 0.02$ .

This too low value suggests that the fit account for the plateau, while it corresponds to a flow regime. In order to determine a reasonable value of  $H_{high}$ , we have first performed a fit assuming  $\beta = 0.32$ , and eliminated the magnetic field range over which the data are too much separated from the fit. A second fit with  $\beta$  taken as a share free parameter was then performed. The obtained result is  $\beta = 0.30 \pm 0.02$ , which is also compatible with the values obtained for GdFeCo.

## CORRELATION LENGTH DEPINNING EXPONENT

At the depinning threshold the typical size of avalanches diverges, as the correlation length  $\xi$ , with the following dependence on the magnetic field:  $\xi \sim (H - H_d)^{-\nu}$  [5]. In addition, if two points on the DW belong to the same avalanche, their instantaneous velocities will be correlated. Therefore, the typical length of avalanches is expected to be proportional to the characteristic length scale in the velocity correlation function [9]. In order to compute the universal exponent of correlation length divergence,  $\nu$ , when  $H \rightarrow H_d(T)$ , we directly estimate  $\xi$  from the velocity correlation function  $C_v$  as the length scale it takes the correlation to halve,  $C_v(x = \xi) = C_0/2$ . Figure 4 shows the velocity correlation function  $C_v(x)$  at different field values for  $T = 20$  K. The horizontal dotted line indicates the value  $C_0/2$  and the points in this line give  $\xi(H)$ . As can be observed in Figure 4 the decay of  $C_v(x)$  is not perfectly exponential. Power-law corrections can be expected for small  $x$  values [9] and some fluctuations are present for large  $x$  values. Nevertheless, we have tested that if we use different values of  $f$  in  $C_v(x = \xi) = fC_0$ , our estimated value for  $\nu$  does not change for  $f$  in the range  $0.2 < f < 0.7$ .

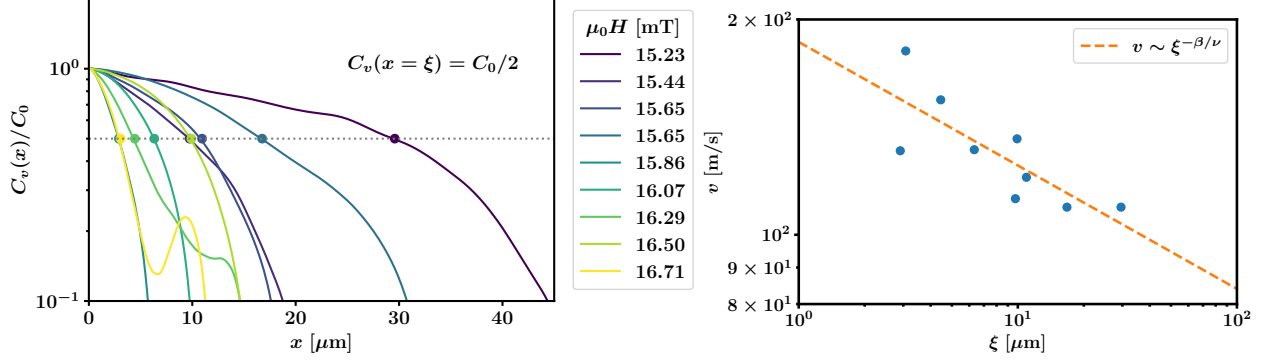

Figure 4. Domain wall velocity fluctuations. Left panel: Correlation length of the velocity for different domain walls at  $T = 20$  K and different field values, as indicated. Right panel:  $v$  vs.  $\xi$  for different external magnetic fields and  $T = 20$  K. Starting from the highest magnetic field used in this experiment, the correlation length increases and the velocity decreases when the magnetic field approaches  $H_d$ . The relation between  $v$  and  $\xi$  can be described using a power-law, as indicated by the dashed line.

## THE LARKIN LENGTH

In the experimental analysis of the different DW motion regimes, the most relevant sample parameters are the *depinning field*  $H_d$  and the characteristic *depinning temperature*  $T_d$ , which set the natural units to measure the fields and temperatures (energies), respectively. Both  $H_d$  and  $T_d$  result from the competition between elasticity and disorder and can be estimated from weak collective pinning Larkin theory [10]. In that picture, the fundamental length scales of the problem are the Larkin length  $L_c$ , in the DW base plane, and the correlation length of the pinning force along the direction of DW displacement,  $\xi_p$ . All other characteristic lengths of the problem can be measured in units of  $L_c$  or  $\xi_p$ . For example, the characteristic size of avalanches at the  $T = 0$  depinning transition is expected to be  $\xi \approx \xi_0(H/H_d - 1)^{-\nu} \approx L_c(H/H_d - 1)^{-\nu}$ . The width of such avalanche is, on the other hand, expected to scale as  $w \approx \xi_p(\xi/\xi_0)^\zeta$ , with  $\zeta$  the depinning roughness exponent. From weak collective pinning theory [8, 10]  $L_c$  relates to  $H_d$  and  $T_d$  as

$$L_c = \frac{k_B T_d}{2M_s H_d s \xi_p}, \quad (2)$$

where  $M_s$  is the saturation magnetization and  $s$  the sample thickness.

Since a domain-wall can only sense spatial variations of the condensation energy larger than its width, the pinning correlation length must satisfy  $\xi_p = \max[\Delta, r_0]$  where  $\Delta$  is the

DW width and  $r_0$  is the characteristic length of the random heterogeneity in the sample. One common problem is that  $r_0$  is in general unknown, as it requires to identify the sample heterogeneity responsible for DW pinning. Fortunately, from Larkin theory we can express  $\xi_p$  in terms of other measurable quantities [8],

$$\xi_p = \left[ (k_B T_d)^2 / (2M_s H_d \sigma s^2) \right]^{1/3}. \quad (3)$$

Given that the sample thickness is  $s = 10$  nm, the DW energy is  $\sigma = 4\Delta K_{eff} = 0.8$  mJ/m<sup>2</sup> (with  $K_{eff} = 20$  kJ/m<sup>3</sup> the effective anisotropy constant), the estimated DW width is [11, 12]  $\Delta = 15$  nm, and in our temperature range,  $H_d \approx 15$  mT,  $M_s \approx 112$  kA/m,  $T_d \approx 30000$  K, we get, using Eq.(3)

$$\xi_p \approx 75 \text{ nm}. \quad (4)$$

Interestingly, this indicates that the range of correlations of the random heterogeneities is larger than  $\Delta$  and thus  $\xi_p \approx r_0$ , as has been also noticed in other materials and for different temperatures [8]. With this estimate of  $\xi_p$ , we finally get the Larkin length using Eq.(2)

$$L_c \approx 165 \text{ nm}, \quad (5)$$

reported in the main text, which is in fair agreement with the scale  $\xi_0$  obtained from the velocity's spatial autocorrelation function.

- 
- [1] S. Bustingorry, A. B. Kolton, and T. Giamarchi, EPL (Europhysics Letters) **81**, 26005 (2008).
  - [2] J. Gorchon, S. Bustingorry, J. Ferré, V. Jeudy, A. B. Kolton, and T. Giamarchi, Phys. Rev. Lett. **113**, 027205 (2014).
  - [3] R. Diaz Pardo, W. Savero Torres, A. B. Kolton, S. Bustingorry, and V. Jeudy, Phys. Rev. B **95** (2017).
  - [4] S. Bustingorry, A. B. Kolton, and T. Giamarchi, Phys. Rev. B **85**, 214416 (2012).
  - [5] E. E. Ferrero, S. Bustingorry, A. B. Kolton, and A. Rosso, C. R. Physique **14**, 641 (2013).
  - [6] V. H. Purrello, J. L. Iguain, A. B. Kolton, and E. A. Jagla, Phys. Rev. E **96**, 022112 (2017).
  - [7] E. E. Ferrero, L. Foini, T. Giamarchi, A. B. Kolton, and A. Rosso, Annu. Rev. Cond. Mat. (in press) (2020), arXiv:2001.11464 [cond-mat.dis-nn].

- [8] V. Jeudy, R. Díaz Pardo, W. Savero Torres, S. Bustingorry, and A. B. Kolton, Phys. Rev. B **98**, 054406 (2018).
- [9] O. Duemmer and W. Krauth, Phys. Rev. E **71**, 061601 (2005).
- [10] A. Larkin and Y. N. Ovchinnikov, Journal of Low Temperature Physics **34**, 409 (1979).
- [11] D.-H. Kim, T. Okuno, S. K. Kim, S.-H. Oh, T. Nishimura, Y. Hirata, Y. Futakawa, H. Yoshikawa, A. Tsukamoto, Y. Tserkovnyak, Y. Shiota, T. Moriyama, K.-J. Kim, K.-J. Lee, and T. Ono, Phys. Rev. Lett. **122**, 127203 (2019).
- [12] E. Haltz, J. Sampaio, S. Krishnia, L. Berges, R. Weil, and A. Mougin, Scientific Reports **10**, 16292 (2020).
